# Supplementary material for: ConvTimeNet: A Deep Hierarchical Fully Convolutional Model for Multivariate Time Series Analysis
Source: arXiv:2403.01493 source file (2024-12-14)
Supplement: Supplementary file 1 [file IJCAI_24_ConvTimeNet_appendix_v1.pdf]

# A Related Work

Time series temporal and cross-variable dependency modeling are crucial issues in time series analysis. In recent years, a variety of modeling techniques have been developed, including those rooted in Convolutional Neural Networks (CNN), Multi-Layer Perceptrons (MLP), and Transformer networks. The CNN-based methods [Zheng *et al.*, 2014; Cui *et al.*, 2016] employ sliding convolutional kernels along the temporal dimension to capture temporal dependency. However, these methods have not achieved ideal results in modeling long-range dependencies due to the limited receptive filed. On the other hand, MLP-based methods [Zeng *et al.*, 2023; Challu *et al.*, 2023] utilize the MLP structure to encode temporal dependencies into the MLP layers. Alternatively, some methods [Das *et al.*, 2023] can integrate covariate information into the network.

The Transformer network, with its ability to capture long-range dependencies and cross variable interactions, is particularly appealing for time series analysis. Consequently, numerous Transformer-based methods have been developed, such as Autoformer [Wu *et al.*, 2021], which utilizes a self-correlation mechanism to capture temporal dependency. Crossformer [Zhang and Yan, 2022], another Transformer-based method, introduces a customized dimension segmentation embedding scheme and an explicit cross-variable attention module designed for forecasting tasks. FormerTime [Cheng *et al.*, 2023], on the other hand, employs hierarchical structure to capture different-scale temporal dependency and variable dependency. Meanwhile, the temporal patching operation [Nie *et al.*, 2022] also significantly improved the performance of the model. Convolutional networks have gradually become less commonly applied in the field of time series analysis.

As modern convolutional techniques continue to evolve, a growing number of convolutional methods are being revisited within the community. For instance, the method [Ding *et al.*, 2022] employs a mechanism of re-parameterization to circumvent issues associated with expanding the convolutional kernel, thereby addressing the issue of receptive field limitation. Additionally, the TimesNet method, introduced recently in [Wu *et al.*, 2022], considers two-dimensional temporal variations generated by periodicities, specifically designed for general tasks in time series analysis.

# B Datasets

We adhere to the same data processing and train-validation-test set split protocol utilized in TimesNet[Wu *et al.*, 2022]. This protocol ensures the strict division of the train, validation, and test datasets based on chronological order, thereby mitigating any data leakage issues. In regard to forecasting settings, we maintain a fixed length of the lookback window at 336 for ETT(ETTh1,ETTh2,ETTm1,ETTm2), Weather, Electricity, Exchange, and Traffic, 104 for Illness dataset. The predicted length, varies within the range of 96,192,336,720 and 24,36,48,60 for Illness. Detailed information about these datasets is provided in the Table 1.

**Time Series Forecasting.** While for time series forecasting, we conduct experiments using nine different datasets, each of which is briefly described as follows: (1) **ETT**[1] encompasses records of oil temperature and load metrics of electricity transformers. The data spans from July 2016 to July 2018, divided into four sub-datasets. (2) **Electricity**[2] comprises electricity usage data from 321 clients. This data covers the period from July 2016 to July 2019. (3) **Exchange**[3] contains daily exchange rates of eight different nations. The data spans from 1990 to 2016. (4) **Traffic**[4] provides hourly traffic volume data on San Francisco freeways, recorded by 862 sensors from 2015 to 2016. (5) **Weather**[5] consists of 21 weather indicators, including air temperature and humidity. The data was collected at 10-minute intervals throughout the year 2021. (6) **Illness** [6] logs the weekly ratio of patients with influenza-like symptoms against the total patients, collected by the Centers for Disease Control and Prevention of the United States from 2002 to 2021.

**Time Series Classification.** The **UEA** [7] archive is recognized as one of the most comprehensive benchmarks for multivariate time series analysis. We carefully pick ten datasets that exhibit a variety of characteristics, including differing numbers and lengths of time series samples, as well as class variety. Each of the ten datasets is briefly described as follows: (1) **ArticularyWordRecognition** contains data collected from multiple native English speakers producing 25 words, to measure the movement of the tongue and lips. (2) **CharacterTrajectories** captures 2858 character samples with three dimensions, to identify one of the 20 characters. (3) **Cricket** records 4 umpires motions while performing 12 cricket signals with 10 repetitions each, aiming to classify the signals based on the accelerometer data. (4) **DuckDuckGeese** is collected from recordings on www.xenocanto.com, to distinguish different bird species. (5) **Epilepsy** records data from 6 healthy participants while performing 4 different activities, and the target is to classify those activities. (6) **EthanolConcentration** records raw spectra of water-and-ethanol solutions in 44 whisky bottles, to determine the alcohol concentration. (7) **FingerMovements** records a normal subject during a no-feedback session, aiming to classify upcoming movements based on EEG (Electroencephalography) recordings from 28 channels. (8) **JapaneseVowels** records 9 Japanese-male speakers saying the vowels 'a' and 'e', to predict the speaker based on the transformed utterances. (9) **PEMS-SF** describes the occupancy rate of car lanes in the San Francisco Bay area freeways, to classify each observed day into the correct day of the week. (10) **SelfRegulationSCP2** records the slow cortical potentials of an ALS (Amyptrophic Lateral Sclerosis) patient, and the task is to predict the direction of cursor movement based on the EEG(Electroencephalography) data.

[1]https://github.com/zhouhaoyi/ETDataset

[2]https://archive.ics.uci.edu/ml/datasets/

[3]https://github.com/laiguokun/multivariate-time-series-data

[4]http://pems.dot.ca.gov

[5]https://www.bgc-jena.mpg.de/wetter/

[6]https://gis.cdc.gov/grasp/fluview/fluportaldashboard.html

[7]https://www.timeseriesclassification.com/dataset.php

Table 1: The dataset descriptions are comprehensive. The variable 'Dim' represents the number of each dataset. The term 'Size' refers to the total number of time points in the (Train, Validation, Test) split. The term 'Series Length' in Time Series Forecasting indicates the future time points to be predicted, and input series length in Time Series Classification. Each dataset in forecasting task comprises four prediction settings. The term 'Frequency' denotes the sampling interval of time points.

| Task | Dataset | Short Name | Dim | Series Length | Dataset Size | Information | Frequency |
|---|---|---|---|---|---|---|---|
| Time Series Forecasting | ETTm1, ETTm2 | ETTm1, ETTm2 | 7 | (96, 192, 336, 720) | (34465, 11521, 11521) | Electricity | 15min |
| | ETTh1, ETTh2 | ETTh1, ETTh2 | 7 | (96, 192, 336, 720) | (8545, 2881, 2881) | Electricity | Hourly |
| | Electricity | Electricity | 321 | (96, 192, 336, 720) | (18317, 2633, 5261) | Electricity | Hourly |
| | Traffic | Traffic | 862 | (96, 192, 336, 720) | (12185, 1757, 3509) | Transportation | Hourly |
| | Weather | Weather | 21 | (96, 192, 336, 720) | (36792, 5271, 10540) | Weather | 10min |
| | Exchange | Exchange | 8 | (96, 192, 336, 720) | (5120, 665, 1422) | Economy | Daily |
| | Illness | Ill | 7 | (24, 36, 48, 60) | (617, 74, 170) | Medicine | Weekly |
| Time Series Classification | ArticularyWordRecognition | AWR | 9 | 144 | (275,0,300) | Motion | 200HZ |
| | CharacterTrajectories | CT | 3 | 182 | (1442,0,1436) | Motion | 200HZ |
| | Cricket | CR | 6 | 1197 | (108,0,72) | HAR | 184HZ |
| | DuckDuckGeese | DDG | 1345 | 270 | (50,0,50) | Audio | 44100HZ |
| | Epilepsy | EP | 3 | 206 | (137,0,138) | HAR | 16HZ |
| | EthanolConcentration | EC | 3 | 1751 | (261,0,263) | Spectro | 0.5nm (of spectrum) |
| | FingerMovements | FM | 28 | 50 | (316,0,100) | EEG | 1000HZ |
| | JapaneseVowels | JV | 12 | 29 | (270,0,370) | Audio | None |
| | PEMS-SF | PEMS | 963 | 144 | (267,0,173) | Transportation | 10 minus |
| | SelfRegulationSCP2 | SRS | 7 | 1152 | (200,0,180) | EEG | 256HZ |

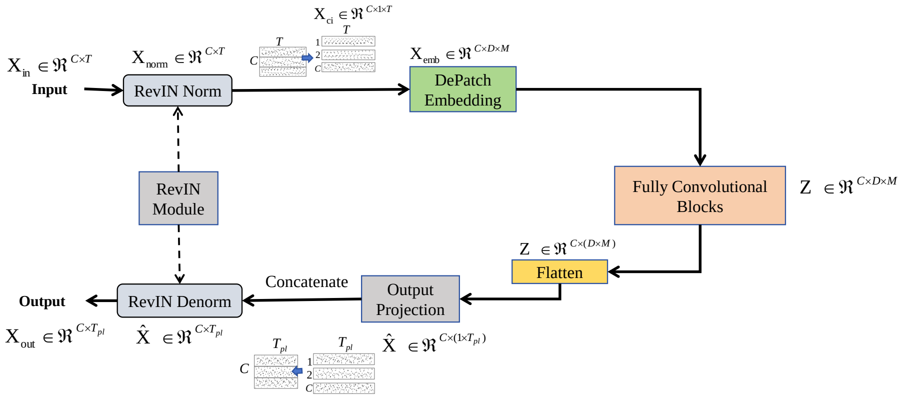


Figure 1: The pipeline of time series forecasting task.

# C Model Configuration

In both tasks, the Deformable patch slicing module employs two convolution layers as its light weight predictor. The design of the fully convolutional block remains uniform, utilizing one layer of deepwise convolution and two layers of pointwise convolution. Additionally, it incorporates learnable residual and reparameter mechanism. Generally, the small kernel size for reparameter is set to either 3 or 5.

**Network for Time Series Forecasting.** For time series forecasting tasks, the pipeline of forward is shown in Figure 1. The input consists of a time series with C variables, each having a specific sequence length $T$. We also employ the series stationarization technique from RevIN [Kim *et al.*, 2021] to mitigate the impact of distribution shifts. To ensure that the model can effectively capture multi-scale information and global receptive field, the number of fully convolution blocks is set to six. For the output prediction layer, we use Flatten and Linear layers as output projection layer, aligning with the setup of PatchTST[Nie *et al.*, 2022]. Denote $X_{out} \in \mathbb{R}^{C \times T_{pl}}$ as output result, where $T_{pl}$ represents the prediction length.

**Network for Time Series Classification.** The pipeline of time series classification task is shown in Figure 2. The input data is a time series comprising C variables, each with a distinct sequence length of T. The number of fully convolution blocks is also generally set to six. For the output layer, we employ max pooling, maintaining consistency with the FormerTime approach [Cheng *et al.*, 2023]. The projection layer, activated with log-softmax, is designed to transform the final representation into the final classification result, $X_{out} \in \mathbb{R}^{C_{nc} \times 1}$, where $C_{nc}$ represents the number of classes.

# D Implement Details

All experiments are conducted using PyTorch [Paszke *et al.*, 2019] on one single NVIDIA 4090 24GB GPU. The model optimization utilizes ADAM [Kingma and Ba, 2014]. For forecasting task, The number of training epochs is fixed at 10. And we use early stopping to prevent model overfitting and set patience into 3. All other hyperparameters and initialization strategies are either derived from the authors of the original works. If no open parameter script is provided, we will set up the experimental parameters according to the default parameter settings, with a learning rate of 0.0001, batch size of 32, and dropout of 0.2. For classification task, the model optimization utilizes ADAM as well. The number of training epochs is fixed at 200. All the baselines reproduced in this study are implemented based on the configurations outlined in the original paper or the official code.

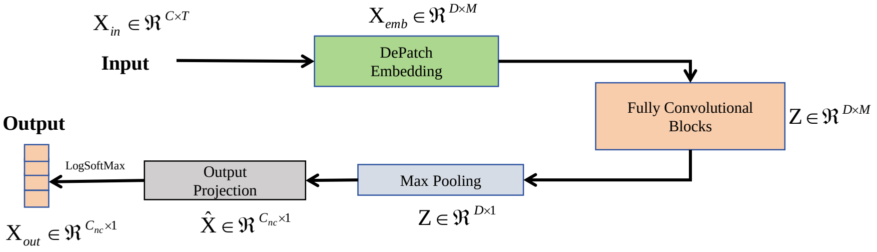


Figure 2: The pipeline of time series classification task.

Table 2: The key parameters of the experiment, where 'DW-Kernel Size' represents the size of the deepwise convolutional kernel in different fully convolutional blocks. 'Patch Size' represents the size of the patch, and 'Stride' represents the step length of the patch window's movement.

| Task | Dataset | DW-Kernel Size | Patch Size | Stride | Hidden Size | Learning Rate | Dropout |
|---|---|---|---|---|---|---|---|
| | ArticularyWordRecognition | 19,19,29,29,37,37 | 32 | | | | |
| | CharacterTrajectories | 7,7,13,13,19,19 | 32 | | | | |
| | Cricket | 19,19,29,29,37,37 | 8 | | | | |
| | DuckDuckGeese | 19,19,29,29,37,37 | 8 | | | | |
| | Epilepsy | 37,37,43,43,53,53 | 4 | | | | |
| Classification | EthanolConcentration | 19,19,29,29,37,37 | 32 | 0.5×Patch Size | 64 | [0.001,0.001] | [0.1,0.1] |
| | FingerMovements | 7,7,13,13,19,19 | 64 | | | | |
| | JapaneseVowels | 7,7,13,13,19,19 | 4 | | | | |
| | PEMS-SF | 19,19,29,29,37,37 | 16 | | | | |
| | SelfRegulationSCP2 | 37,37,43,43,53,53 | 32 | | | | |
| | ETTh1 | 9,11,15,21,29,39 | 32 | | | | |
| | ETTh2 | 5,7,9,11,13,15 | 32 | | | | |
| | ETTm1 | 9,11,15,21,29,39 | 32 | | | | |
| | ETTm2 | 11,15,19,25,33,43,55 | 32 | | | | |
| Forecasting | Traffic | 15,17,21,27,35,55 | 32 | 0.5×Patch Size | 64 | [0.0001,0.005] | [0.1,0.5] |
| | Weather | 11,15,19,25,33,43,55 | 32 | | | | |
| | Electricity | 11,15,21,29,39,51 | 32 | | | | |
| | Exchange Rate | 9,11,15,21,29,39 | 32 | | | | |
| | Illness | 9,11,15,21,29,39 | 16 | | | | |

**Hyper-parameter.** To ensure the reproducibility of the experiment, we have listed the hyperparameter settings for two tasks in the Table 2. The main parameters include the number of fully convolutional blocks, the varying kernel size within different blocks, the setting of the hidden size, and the range of adjustment for dropout and learning rate. In addition, we have provided experimental scripts in the open-source code, allowing users to run it directly.

In the classification task, we adopted a three-stages hierarchical structure. Each stage contains two fully convolutional blocks with equal kernel sizes. We use a six-stages hierarchy in forecasting tasks, with each stage containing one fully convolutional block. The trend of kernel changes in the both task is clearly from small to large. Meanwhile, we use different sizes of patch windows for different data sets, and uniformly set the sliding step of the window to half the size of the patch, ensuring that there is an overlap of half of a continuous patch block. We also verify the effectiveness of this patch setting through experiments.

# E More Experimental Results

## E.1 The Ablation of Learnable Residual

To mitigate the risk of overfitting potentially associated with the extensive stacking of fully convolutional blocks, we introduced the concept of learnable residual within the architecture of ConvTimeNet. This feature is specifically utilized to balance the model's complexity with its learning capacity. To empirically evaluate the impact of learnable residual, we conduct a series of ablation studies across ten distinct datasets, focusing on classification tasks. The results of these studies are illuminating in Table 3. On average, the incorporation of learnable residual into ConvTimeNet led to a 4% enhancement in model performance. This improvement can likely be attributed to the learnable residual, which can dynamically adjust the contribution of each layer to the final output, enabling the model to effectively capture and represent more complex patterns in the data without succumbing to overfitting.

Table 3: Experimental results w.r.t. studying the effectiveness of learnable redsidual.

| | W/ Learnable Redsidual | | W/O Learnable Residual | |
|---|---|---|---|---|
| Metric | Accuracy | F1 Score | Accuracy | F1 Score |
| AWR | **0.987** | **0.987** | 0.986 | 0.986 |
| CR | **0.986** | **0.986** | 0.949 | 0.948 |
| CT | **0.995** | **0.995** | **0.995** | **0.995** |
| EC | **0.338** | 0.249 | 0.331 | **0.266** |
| EP | **0.988** | **0.988** | 0.978 | 0.979 |
| FM | **0.680** | **0.677** | 0.627 | 0.626 |
| JV | **0.990** | **0.990** | 0.989 | **0.990** |
| PEMS | 0.830 | 0.823 | **0.873** | **0.870** |
| SRS | 0.596 | 0.594 | **0.624** | **0.621** |
| DDG | **0.660** | **0.652** | 0.467 | 0.415 |

## E.2 Performance Comparision of Varying Layer Depth

To validate the impact of the number of building blocks, we conducted experiments on ten datasets for classification tasks,

Table 4: Experimental results w.r.t. studying the hyperparameter sensitivity of the number of fully convolutional blocks.

| Depth | 3 Layers | | 6 Layers | | 9 Layers | |
|---|---|---|---|---|---|---|
| Metric | Accuracy | F1 Score | Accuracy | F1 Score | Accuracy | F1 Score |
| AWR | 0.978 | 0.978 | 0.987 | 0.987 | **0.988** | **0.988** |
| CR | 0.977 | 0.977 | **0.986** | **0.986** | 0.968 | 0.967 |
| CT | 0.992 | 0.992 | **0.995** | **0.995** | 0.994 | 0.994 |
| EC | 0.331 | **0.285** | 0.338 | 0.249 | **0.345** | 0.282 |
| EP | 0.978 | 0.978 | **0.988** | **0.988** | 0.986 | 0.986 |
| FM | 0.673 | 0.671 | **0.680** | **0.677** | 0.647 | 0.647 |
| JV | **0.994** | **0.994** | 0.990 | 0.990 | 0.991 | 0.991 |
| PEMS | 0.825 | 0.817 | **0.830** | **0.823** | 0.804 | 0.794 |
| SRS | 0.576 | 0.567 | **0.596** | **0.594** | 0.563 | 0.562 |
| DDG | 0.560 | 0.523 | **0.660** | **0.652** | 0.630 | 0.623 |

varying the number of fully convolutional blocks. The results show in Table 4 indicate that stacking building blocks mostly enhances model performance. However, in most datasets, clear overfitting occurs when the number of blocks reaches nine. This could be attributed to the relatively smaller data volumes in classification tasks, which may hinder the model's ability to undergo sufficient training.

### E.3 Impact of Patch Size

The patch slicing operation is a crucial aspect of ConvTimeNet, as it determines the richness of semantic information in time series data. Therefore, we conduct experiments to assess the sensitivity of patch size on three datasets for forecasting tasks. The experimental results are presented in the Table 5, where $P$ denotes the patch length, and $S$ represents the stride of the patch window. The findings indicate that a bigger patch length of 32 typically achieves superior performance in most cases. Additionally, setting the stride to half the slice length can also enhance model performance. This improvement might be attributed to the general overlap between patches, which ensures the continuity of time series semantics. Furthermore, capturing more patches within a certain length of time series data ensures a richer semantic understanding.

### E.4 The Ablation of Re-parameter Mechanism

Within the fully convolutional block of our model, a re-parameter mechanism is integrated, which not only aids in gathering detailed feature insights with small kernel size but also greatly enable the model to expand the kernel size to be larger. To empirically evaluate the efficacy of this re-parameter mechanism, a series of ablation studies are undertaken across a variety of classification task datasets. As the result show in Table 6. Implementing the re-parameter mechanism resulted in an approximate 6% enhancement in the model's accuracy for classification tasks. The experimental results thus strongly underscore the pivotal role that the re-parameter mechanism plays in elevating the overall performance of the model. Additionally, it is observed from the data that simply increasing the kernel size does not necessarily enhance the model's performance in scenarios where the re-parameter mechanism is not utilized.

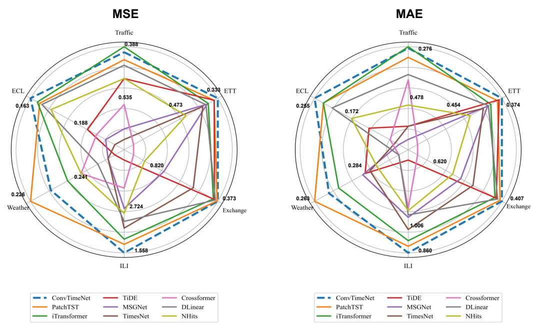


Figure 3: Model performance in time series forecasting task.

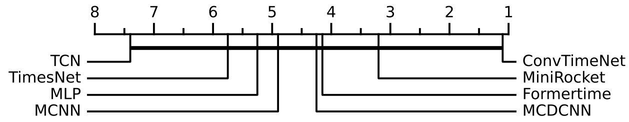


Figure 4: Critical difference diagram over the mean ranks of ConvTimeNet, baseline methods of classification task.

## F Case Study Analysis

We present visual representations for time series forecasting in Figure 5. These visual representations provide a clear comparison among various models. The study randomly selects a sample from the test dataset as input and plots the prediction results in all models. It can be intuitively observed from the chart that the prediction trend of ConvTimeNet is more stable compared to DLinear and NHits. Although MSGNet also shows relative stability, the prediction trend of ConvTimeNet is more in line with ground truth.

## G Full Results

In this section, we supplement the full experimental results of two tasks and include relevant analysis figures.

### G.1 Time Series Forecasting

ConvTimeNet has achieved state-of-the-art performance in time series prediction tasks, as can be seen directly from the Figure 3 in comparison with various datasets. The statistic in the figure is the average of all methods across four different prediction length settings on each dataset.

### G.2 Time Series Classification

Figure 4 illustrates the critical difference diagram of classification task as presented in [Demšar, 2006]. Due to space constraints, we only placed the Accuracy performance of the classification task in the main text. The complete experimental results are shown in the Table 7. We supplement the experimental results of effectiveness over the hierarchical structure in Table 8.

Table 5: Experimental results w.r.t. studying the hyperparameter sensitivity of patch size. $P$ denotes the slice length, and $S$ represents the stride of the patch window.

| Window Size | | P=32,S=16 | | P=32,S=32 | | P=16,S=8 | | P=16,S=16 | | P=8,S=4 | | P=8,S=8 | |
|---|---|---|---|---|---|---|---|---|---|---|---|---|---|
| Metric | | MSE | MAE | MSE | MAE | MSE | MAE | MSE | MAE | MSE | MAE | MSE | MAE |
| ETTh1 | 96 | 0.369 | 0.395 | 0.375 | 0.400 | **0.368** | **0.393** | 0.369 | 0.395 | 0.369 | 0.394 | **0.368** | **0.393** |
| | 192 | **0.406** | 0.414 | 0.411 | 0.418 | **0.406** | **0.413** | **0.406** | 0.414 | 0.407 | 0.414 | **0.406** | **0.413** |
| | 336 | **0.405** | **0.420** | 0.407 | 0.425 | **0.405** | **0.420** | **0.405** | 0.422 | 0.410 | 0.425 | **0.405** | 0.421 |
| | 720 | 0.442 | **0.457** | **0.441** | 0.458 | 0.446 | 0.459 | 0.443 | **0.457** | 0.450 | 0.462 | 0.445 | 0.458 |
| ETTm1 | 96 | **0.292** | **0.345** | **0.292** | **0.345** | 0.297 | 0.349 | 0.297 | 0.349 | 0.301 | 0.352 | 0.296 | 0.349 |
| | 192 | **0.329** | **0.368** | 0.330 | 0.369 | 0.336 | 0.375 | 0.336 | 0.375 | 0.343 | 0.380 | 0.333 | 0.372 |
| | 336 | **0.363** | **0.390** | 0.365 | 0.393 | 0.372 | 0.398 | 0.372 | 0.398 | 0.376 | 0.403 | 0.370 | 0.399 |
| | 720 | **0.427** | 0.428 | **0.427** | **0.427** | 0.435 | 0.434 | 0.435 | 0.434 | 0.440 | 0.437 | 0.433 | 0.432 |
| Exchange | 96 | **0.086** | **0.204** | **0.086** | **0.204** | 0.088 | 0.207 | 0.088 | 0.207 | 0.088 | 0.208 | 0.088 | 0.207 |
| | 192 | 0.184 | 0.303 | **0.181** | **0.301** | **0.181** | 0.302 | **0.181** | 0.302 | 0.189 | 0.307 | 0.185 | 0.306 |
| | 336 | 0.341 | 0.421 | **0.335** | 0.418 | 0.343 | 0.425 | 0.343 | 0.425 | **0.335** | **0.417** | 0.339 | 0.421 |
| | 720 | **0.879** | **0.701** | 1.014 | 0.765 | 0.881 | 0.704 | 0.881 | 0.704 | 0.890 | 0.707 | 0.895 | 0.709 |

Table 6: The ablation results of re-parameter mechanism.

| | W/ Reparameter | | | | | | W/O Reparameter | | | | | |
|---|---|---|---|---|---|---|---|---|---|---|---|---|
| Metric | Accuracy | F1 Score | Accuracy | F1 Score | Accuracy | F1 Score | Accuracy | F1 Score | Accuracy | F1 Score | Accuracy | F1 Score |
| Setting | [7,7,7,7,7,7] | | [7,7,7,13,13,13] | | [7,7,13,13,19,19] | | [7,7,7,7,7,7] | | [7,7,7,13,13,13] | | [7,7,13,13,19,19] | |
| CT | 0.992 | 0.991 | **0.995** | **0.995** | **0.995** | **0.995** | 0.992 | 0.991 | 0.992 | 0.992 | 0.991 | 0.990 |
| FM | 0.640 | 0.632 | 0.643 | 0.641 | **0.680** | **0.677** | 0.623 | 0.619 | 0.637 | 0.635 | 0.630 | 0.625 |
| JV | **0.990** | 0.989 | 0.987 | 0.987 | **0.990** | **0.990** | 0.981 | 0.980 | 0.981 | 0.981 | 0.982 | 0.981 |
| Setting | [19,19,19,19,19,19] | | [19,19,19,29,29,29] | | [19,19,29,29,37,37] | | [19,19,19,19,19,19] | | [19,19,19,29,29,29] | | [19,19,29,29,37,37] | |
| CR | 0.982 | 0.981 | 0.977 | 0.976 | **0.986** | **0.986** | 0.977 | 0.976 | **0.986** | **0.986** | 0.963 | 0.960 |
| AWR | 0.984 | 0.984 | 0.982 | 0.982 | **0.987** | **0.987** | 0.981 | 0.981 | 0.979 | 0.979 | 0.978 | 0.978 |
| EC | **0.347** | 0.267 | 0.338 | 0.273 | 0.338 | 0.249 | 0.321 | 0.286 | 0.321 | **0.296** | 0.295 | 0.274 |
| PEMS | 0.803 | 0.797 | 0.847 | 0.843 | 0.830 | 0.823 | 0.846 | 0.841 | 0.852 | 0.845 | **0.856** | **0.852** |
| DDG | 0.573 | 0.540 | 0.580 | 0.578 | **0.660** | **0.652** | 0.513 | 0.500 | 0.567 | 0.544 | 0.540 | 0.509 |
| Setting | [37,37,37,37,37,37] | | [37,37,37,43,43,43] | | [37,37,43,43,53,53] | | [37,37,37,37,37,37] | | [37,37,37,43,43,43] | | [37,37,43,43,53,53] | |
| EP | **0.988** | **0.988** | 0.981 | 0.981 | **0.988** | **0.988** | 0.961 | 0.959 | 0.978 | 0.977 | 0.966 | 0.965 |
| SRS | 0.585 | 0.579 | 0.580 | 0.562 | **0.596** | **0.594** | 0.567 | 0.564 | 0.569 | 0.547 | 0.552 | 0.516 |

Figure 5: The visualization of ETTh1 predictions, generated by various models under the input-336-predict-336 setting, is presented. The black lines represent the ground truth, while the orange lines represent the predicted values.

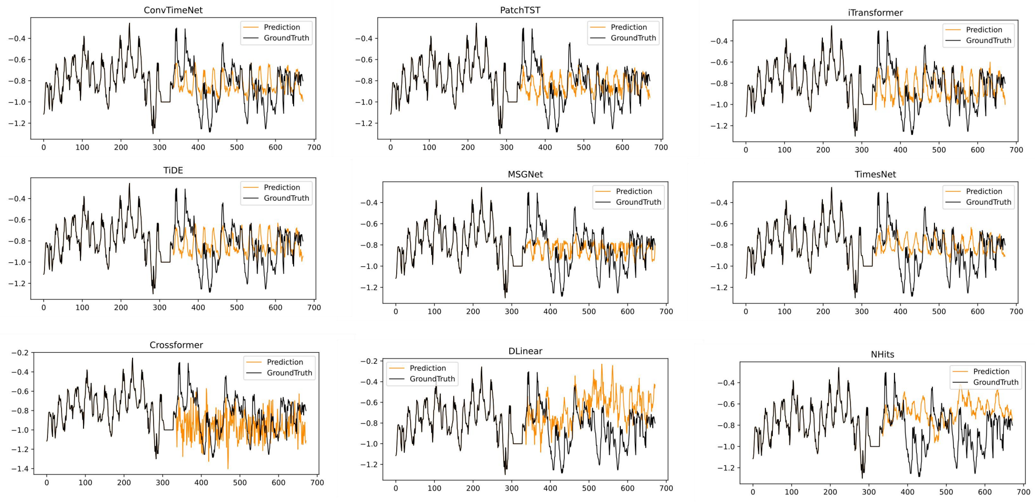

Table 7: Full results of time series classification task, in terms of Accuracy and F1 score. Noted that − indicates that the model cannot run due to the issue of being out of memory.

| Metric | Datasets | ConvTimeNet | FormerTime | TimesNet | MiniRocket | TST | MLP | TCN | MCNN | MCDCNN |
|---|---|---|---|---|---|---|---|---|---|---|
| Accuracy | AWR | **0.987** | 0.978 | 0.980 | 0.972 | 0.980 | 0.960 | 0.884 | 0.977 | 0.980 |
| | CR | **0.986** | 0.917 | 0.889 | 0.981 | 0.898 | 0.935 | 0.868 | 0.917 | 0.870 |
| | CT | **0.995** | 0.992 | 0.984 | 0.987 | 0.990 | 0.955 | 0.968 | 0.991 | 0.988 |
| | EC | **0.338** | 0.312 | 0.287 | 0.327 | - | 0.309 | 0.299 | 0.293 | 0.298 |
| | EP | 0.988 | 0.952 | 0.902 | **0.993** | 0.901 | 0.961 | 0.942 | 0.961 | 0.971 |
| | FM | **0.680** | 0.650 | 0.610 | 0.638 | 0.580 | 0.607 | 0.580 | 0.597 | 0.617 |
| | JV | **0.990** | 0.986 | 0.981 | 0.987 | 0.986 | 0.983 | 0.974 | 0.977 | 0.978 |
| | PEMS | **0.830** | 0.173 | 0.728 | 0.795 | 0.778 | 0.761 | 0.669 | 0.804 | 0.792 |
| | SRS | **0.596** | 0.572 | 0.542 | 0.564 | 0.541 | 0.546 | 0.507 | 0.574 | 0.565 |
| | DDG | **0.660** | 0.240 | 0.400 | 0.620 | 0.340 | 0.280 | 0.200 | 0.213 | 0.624 |
| F1 Score | AWR | **0.987** | 0.978 | 0.980 | 0.970 | 0.980 | 0.959 | 0.883 | 0.977 | 0.980 |
| | CR | **0.986** | 0.918 | 0.886 | 0.980 | 0.890 | 0.929 | 0.861 | 0.906 | 0.863 |
| | CT | **0.995** | 0.991 | 0.983 | 0.986 | 0.989 | 0.949 | 0.966 | 0.990 | 0.987 |
| | EC | 0.249 | 0.261 | 0.181 | **0.298** | - | 0.248 | 0.221 | 0.234 | 0.241 |
| | EP | 0.988 | 0.950 | 0.896 | **0.990** | 0.899 | 0.961 | 0.940 | 0.960 | 0.971 |
| | FM | **0.677** | 0.628 | 0.604 | 0.620 | 0.568 | 0.602 | 0.572 | 0.586 | 0.605 |
| | JV | **0.990** | 0.984 | 0.980 | 0.988 | 0.986 | 0.982 | 0.975 | 0.974 | 0.976 |
| | PEMS | **0.823** | 0.042 | 0.720 | 0.786 | 0.771 | 0.747 | 0.613 | 0.799 | 0.788 |
| | SRS | **0.594** | 0.579 | 0.507 | 0.515 | 0.487 | 0.516 | 0.371 | 0.573 | 0.565 |
| | DDG | **0.652** | 0.113 | 0.290 | 0.622 | 0.227 | 0.148 | 0.067 | 0.092 | 0.600 |

Table 8: Full results of studying the effectiveness of deep hierarchical architecture in terms of Accuracy and F1 score.

| Metric | Hierarchy | | One stage | | | Two Stages | | Three Stages |
|---|---|---|---|---|---|---|---|---|
| Accuracy | Setting | [7,7,7,7,7,7] | [13,13,13,13,13,13] | [19,19,19,19,19,19] | [7,7,7,13,13,13] | [7,7,7,19,19,19] | [13,13,13,19,19,19] | [7,7,13,13,19,19] |
| | CT | 0.992 | 0.994 | **0.995** | **0.995** | 0.993 | **0.995** | **0.995** |
| | FM | 0.640 | **0.680** | 0.653 | 0.643 | 0.660 | 0.630 | **0.680** |
| | JV | 0.990 | 0.990 | 0.988 | 0.987 | 0.991 | **0.992** | 0.990 |
| | Setting | [19,19,19,19,19,19] | [29,29,29,29,29,29] | [37,37,37,37,37,37] | [19,19,19,29,29,29] | [19,19,19,37,37,37] | [29,29,29,37,37,.37] | [19,19,29,29,37,37] |
| | CR | 0.982 | 0.977 | 0.982 | 0.977 | 0.958 | 0.972 | **0.986** |
| | AWR | 0.984 | 0.982 | 0.975 | 0.982 | 0.980 | 0.979 | **0.987** |
| | EC | **0.347** | 0.345 | 0.342 | 0.338 | 0.340 | 0.337 | 0.338 |
| | PEMS | 0.803 | 0.807 | 0.829 | **0.847** | 0.819 | 0.807 | 0.830 |
| | DDG | 0.573 | 0.560 | 0.500 | 0.580 | 0.513 | 0.513 | **0.660** |
| | Setting | [37,37,37,37,37,37] | [43,43,43,43,43,43] | [53,53,53,53,53,53] | [37,37,37,43,43,43] | [37,37,37,53,53,53] | [43,43,43,53,53,53] | [37,37,43,43,53,53] |
| | EP | **0.988** | 0.983 | 0.981 | 0.981 | 0.978 | 0.976 | **0.988** |
| | SRS | 0.585 | 0.570 | 0.589 | 0.580 | 0.582 | 0.589 | **0.596** |
| F1 Score | Setting | [7,7,7,7,7,7] | [13,13,13,13,13,13] | [19,19,19,19,19,19] | [7,7,7,13,13,13] | [7,7,7,19,19,19] | [13,13,13,19,19,19] | [7,7,13,13,19,19] |
| | CT | 0.991 | 0.994 | **0.995** | **0.995** | 0.993 | 0.994 | **0.995** |
| | FM | 0.632 | 0.676 | 0.651 | 0.641 | 0.657 | 0.629 | **0.677** |
| | JV | 0.989 | 0.990 | 0.988 | 0.987 | **0.993** | 0.991 | 0.990 |
| | Setting | [19,19,19,19,19,19] | [29,29,29,29,29,29] | [37,37,37,37,37,37] | [19,19,19,29,29,29] | [19,19,19,37,37,37] | [29,29,29,37,37,.37] | [19,19,29,29,37,37] |
| | CR | 0.981 | 0.977 | 0.981 | 0.976 | 0.958 | 0.972 | **0.986** |
| | AWR | 0.984 | 0.982 | 0.974 | 0.982 | 0.980 | 0.979 | **0.987** |
| | EC | 0.267 | **0.304** | 0.298 | 0.273 | 0.267 | 0.265 | 0.249 |
| | PEMS | 0.797 | 0.798 | 0.819 | **0.843** | 0.812 | 0.801 | 0.823 |
| | DDG | 0.540 | 0.527 | 0.496 | 0.578 | 0.521 | 0.452 | **0.652** |
| | Setting | [37,37,37,37,37,37] | [43,43,43,43,43,43] | [53,53,53,53,53,53] | [37,37,37,43,43,43] | [37,37,37,53,53,53] | [43,43,43,53,53,53] | [37,37,43,43,53,53] |
| | EP | **0.988** | 0.983 | 0.981 | 0.981 | 0.979 | 0.975 | **0.988** |
| | SRS | 0.579 | 0.569 | 0.579 | 0.562 | 0.569 | 0.563 | **0.594** |

## References


[Challu *et al.*, 2023] Cristian Challu, Kin G Olivares, Boris N Oreshkin, Federico Garza Ramirez, Max Mergenthaler Canseco, and Artur Dubrawski. Nhits: Neural hierarchical interpolation for time series forecasting. In *Proceedings of the AAAI Conference on Artificial Intelligence*, volume 37, pages 6989–6997, 2023.

[Cheng *et al.*, 2023] Mingyue Cheng, Qi Liu, Zhiding Liu, Zhi Li, Yucong Luo, and Enhong Chen. Formertime: Hierarchical multi-scale representations for multivariate time series classification. *arXiv preprint arXiv:2302.09818*, 2023.

[Cui *et al.*, 2016] Zhicheng Cui, Wenlin Chen, and Yixin Chen. Multi-scale convolutional neural networks for time series classification. *arXiv preprint arXiv:1603.06995*, 2016.

[Das *et al.*, 2023] Abhimanyu Das, Weihao Kong, Andrew Leach, Rajat Sen, and Rose Yu. Long-term forecasting with tide: Time-series dense encoder. *arXiv preprint arXiv:2304.08424*, 2023.

[Demšar, 2006] Janez Demšar. Statistical comparisons of classifiers over multiple data sets. *The Journal of Machine learning research*, 7:1–30, 2006.

[Ding *et al.*, 2022] Xiaohan Ding, Xiangyu Zhang, Jungong Han, and Guiguang Ding. Scaling up your kernels to 31x31: Revisiting large kernel design in cnns. In *Proceedings of the IEEE/CVF conference on computer vision and pattern recognition*, pages 11963–11975, 2022.

[Kim *et al.*, 2021] Taesung Kim, Jinhee Kim, Yunwon Tae, Cheonbok Park, Jang-Ho Choi, and Jaegul Choo. Reversible instance normalization for accurate time-series forecasting against distribution shift. In *International Conference on Learning Representations*, 2021.

[Kingma and Ba, 2014] Diederik P Kingma and Jimmy Ba. Adam: A method for stochastic optimization. *arXiv preprint arXiv:1412.6980*, 2014.

[Nie *et al.*, 2022] Yuqi Nie, Nam H Nguyen, Phanwadee Sinthong, and Jayant Kalagnanam. A time series is worth 64 words: Long-term forecasting with transformers. *arXiv preprint arXiv:2211.14730*, 2022.

[Paszke *et al.*, 2019] Adam Paszke, Sam Gross, Francisco Massa, Adam Lerer, James Bradbury, Gregory Chanan, Trevor Killeen, Zeming Lin, Natalia Gimelshein, Luca Antiga, et al. Pytorch: An imperative style, high-performance deep learning library. *Advances in neural information processing systems*, 32, 2019.

[Wu *et al.*, 2021] Haixu Wu, Jiehui Xu, Jianmin Wang, and Mingsheng Long. Autoformer: Decomposition transformers with auto-correlation for long-term series forecasting. *Advances in Neural Information Processing Systems*, 34:22419–22430, 2021.

[Wu *et al.*, 2022] Haixu Wu, Tengge Hu, Yong Liu, Hang Zhou, Jianmin Wang, and Mingsheng Long. Timesnet: Temporal 2d-variation modeling for general time series analysis. *arXiv preprint arXiv:2210.02186*, 2022.

[Zeng *et al.*, 2023] Ailing Zeng, Muxi Chen, Lei Zhang, and Qiang Xu. Are transformers effective for time series forecasting? In *Proceedings of the AAAI conference on artificial intelligence*, volume 37, pages 11121–11128, 2023.

[Zhang and Yan, 2022] Yunhao Zhang and Junchi Yan. Crossformer: Transformer utilizing cross-dimension dependency for multivariate time series forecasting. In *The Eleventh International Conference on Learning Representations*, 2022.

[Zheng *et al.*, 2014] Yi Zheng, Qi Liu, Enhong Chen, Yong Ge, and J Leon Zhao. Time series classification using multi-channels deep convolutional neural networks. In *International conference on web-age information management*, pages 298–310. Springer, 2014.
